# Supplementary material for: A Lie bracket approximation approach to distributed optimization over directed graphs
Source: arXiv:1711.05486 ancillary file (2019-06-05)
Supplement: Supplementary file 1 [file reformulationLiuSussmann.pdf]

Technical report

# Approximating sequences for the excitation of iterated Lie brackets

A reformulation of the Liu/Sussmann algorithm

Simon Michalowsky, Bahman Gharesifard, Christian Ebenbauer

**Abstract** We consider the problem of approximating the trajectories of a so-called extended system of the form  $\dot{x} = f_0(x) + \sum_{i=1}^r v_{B_i}(t)B_i(x)$ , where the  $B_i$  are Lie brackets of a set of vector fields  $\phi_1, \phi_2, \dots, \phi_M$ , by trajectories of systems of the form  $\dot{x}^\sigma = f_0(x^\sigma) + \sum_{k=1}^M \phi_k(x^\sigma)U_k^\sigma(t)$ , where  $U_k^\sigma$  are input functions to be designed in such a way that, for increasing  $\sigma$ ,  $x^\sigma(t)$  uniformly converges to  $x(t)$ . We present a more algorithmic reformulation of the algorithm proposed in [3] for the computation of suitable approximating inputs  $U_k^\sigma$  of highly oscillatory type and discuss possible simplifications as well as extensions.

## 1. Motivation

Consider a family of nonlinear input-affine systems parametrized by  $\sigma > 0$  in the form

$$\dot{x}^\sigma = \sum_{k=1}^M \phi_k(x^\sigma)U_k^\sigma(t), \quad (1)$$

where  $\phi_k : \mathbb{R}^n \rightarrow \mathbb{R}^n$  are given and  $U_k^\sigma : \mathbb{R} \rightarrow \mathbb{R}$  are the to be designed control inputs. In many applications, especially in the motion planning problem for nonholonomic (mechanical) systems, it is desired to design the control inputs in such a way that the trajectories of (1) follow a given path. From nonlinear controllability analysis it is well-known that all trajectories (1) can exhibit are trajectories of the so-called extended

system

$$\dot{x} = \sum_{i=1}^r v_{B_i}(t) B_i(x), \quad (2)$$

where the  $B_i$  are Lie brackets of the vector fields  $\phi_1, \phi_2, \dots, \phi_M$ . Thus, closely related to the motion planning problem is the problem of exciting certain Lie brackets in (2). This problem also has several other interesting applications such as extremum seeking [1] or distributed algorithms [2, 4, 5]. All these problems have in common that we have a system in the form (2) given and the goal is to find a corresponding system in the form (1) such that the trajectories of (1) converge to those of (2) as  $\sigma$  increases. While there exist many results in the literature on the motion planning problem, this closely related but still different problem has not been dealt with a lot. In fact, to the best of our knowledge, the only work solving this problem in its general form is given by [3], [6], where the authors present an algorithm to design suitable control inputs  $U_k^\sigma$  of highly oscillatory type. However, partly caused by its generality, the algorithm is quite intricate and thus not easily to be implemented. Further, it involves a lot of free parameters which heavily affect the behavior of (1). Hence, the goal of this technical note is to present a reformulated version of the algorithm, discuss particular parameter choices and, in particular, present a simplified algorithm that exploits structural properties of the vector fields  $\phi_k$  in (1). The last point is of particular interest since this simplification has interesting applications in [2, 4, 5] which are our main motivation for this technical note.

## 2. Notation

Apart from standard notation we make use of several expressions that are related to Lie brackets of vector fields. Given two continuously differentiable vector fields  $f_1, f_2 : \mathbb{R}^n \rightarrow \mathbb{R}^n$ , the Lie bracket  $[\cdot, \cdot] : \mathcal{C}^1 \times \mathcal{C}^1 \rightarrow \mathcal{C}$  of  $f_1$  and  $f_2$  evaluated at  $x$  is defined to be

$$[f_1, f_2](x) := \frac{\partial f_2}{\partial x}(x) f_1(x) - \frac{\partial f_1}{\partial x}(x) f_2(x). \quad (3)$$

For a set of vector fields  $\Phi = \{f_1, f_2, \dots, f_p\}$ ,  $f_i : \mathbb{R}^n \rightarrow \mathbb{R}^n$ ,  $f_i \in \mathcal{C}^1$ , we denote by  $\mathcal{LA}(\Phi)$  the set of Lie brackets generated by  $\Phi$ . For an (iterated) Lie bracket  $B = [B_1, B_2]$ ,  $B_1, B_2 \in \mathcal{LA}(\Phi)$ , we then let  $\text{left}(B) = B_1$ ,  $\text{right}(B) = B_2$  denote the left and right factor of  $B$ , respectively. We further define the degree of a Lie bracket  $B \in \mathcal{LA}(\Phi)$  as  $\delta(B) = \tilde{\delta}_\Phi$  and the degree of the  $k$ th vector field as  $\delta_k(B) = \tilde{\delta}_{\{f_k\}}$  where

$$\tilde{\delta}_S(B) = \begin{cases} 1 & \text{if } B \in S \\ \delta(\text{left}(B)) + \delta(\text{right}(B)) & \text{otherwise,} \end{cases} \quad (4)$$

with  $\mathcal{S} \subseteq \Phi$ . Additionally, we let  $\text{Re} : \mathbb{C} \rightarrow \mathbb{R}$  denote the real part of a complex number and  $\text{Im} : \mathbb{C} \rightarrow \mathbb{R}$  its imaginary part.

### 3. Problem formulation

Let  $\Phi = \{\phi_1, \phi_2, \dots, \phi_M\}$ ,  $\phi_i : \mathbb{R}^n \rightarrow \mathbb{R}^n$ ,  $\phi_i$  sufficiently smooth, be a set of vector fields and let  $\mathcal{PH}(\Phi) = (\mathbb{P}, \prec)$  denote a corresponding P. Hall basis (see [Definition 4](#)). Consider an extended system of the following form

$$\dot{x} = f_0(x) + \sum_{B \in \mathcal{B}} v_B(t) B(x), \quad x(0) = x_0, \quad (5)$$

where  $f_0 : \mathbb{R}^n \rightarrow \mathbb{R}^n$ ,  $f_0 \in \mathcal{C}^1$ ,  $\mathcal{B} \subset \mathbb{P}$  is the set of brackets we want to excite and  $v_B : \mathbb{R} \rightarrow \mathbb{R}$ ,  $v_B \in \mathcal{C}^1$  is the time-varying coefficient corresponding to the bracket  $B$ . The goal is to determine input sequences  $U_k^\sigma : \mathbb{R} \rightarrow \mathbb{R}$  such that the trajectories of

$$\dot{x}^\sigma = f_0(x^\sigma) + \sum_{k=1}^M \phi_k(x^\sigma) U_k^\sigma(t), \quad x^\sigma(0) = x_0, \quad (6)$$

uniformly converge to those of (5). To this end, we follow the algorithm presented in [3], [6] and sum it up in a more algorithmic way in the following. The algorithm relies on a “superposition principle”, i.e., we group the brackets  $B \in \mathcal{B}$  into equivalence classes, which we later denote by  $E$ , associate to each class an input  $U_{k,E}^\sigma$  and then add them up as

$$U_k^\sigma(t) = \sum_{E \in \mathcal{E}} U_{k,E}^\sigma(t), \quad k = 1, 2, \dots, M, \quad (7)$$

where  $\mathcal{E}$  is the set of all equivalence classes in  $\mathcal{B}$ . Here, we the equivalence relation on the brackets is defined as follows:

**Definition 1.** Let  $\mathcal{PH}(\Phi) = (\mathbb{P}, \prec)$  be a P. Hall basis of  $\Phi = \{\phi_1, \dots, \phi_M\}$  and let  $\delta_k(B)$  denote the degree of the vector field  $\phi_k$  in the bracket  $B \in \mathcal{PH}$ . We say that two brackets  $B_1, B_2 \in \mathbb{P}$  are equivalent,  $B_1 \sim B_2$ , if  $\delta_k(B_1) = \delta_k(B_2)$  for all  $k = 1, \dots, M$ .

In a nutshell, this means that two brackets are equivalent if each vector field appears the same number of times, but possibly in a different order. We then define the equivalence class corresponding to the bracket  $B \in \mathbb{P}$  as

$$E(B) = \{\tilde{B} \in \mathbb{P} : \tilde{B} \sim B\} \quad (8)$$

and for any equivalence class  $E$  we define  $\delta(E) = \delta(B)$ ,  $\delta_k(E) = \delta_k(B)$ , where  $B$  is any

bracket in  $E$ . For each class  $E \in \mathcal{E}$  we then let the corresponding input take the form

$$U_{k,E}^\sigma(t) = \begin{cases} \eta_{k,0}(t) & \text{if } \delta(E) = 1, \delta_k(E) = 1 \\ 2\sqrt{\sigma}\text{Re}(\eta_{E,k}(\omega_E, t)e^{j\sigma\omega_E t}) & \text{if } \delta(E) = 2, \delta_k(E) = 1 \\ 2\sigma\frac{N-1}{N} \sum_{\rho=1}^{|E|} \sum_{\omega \in \Omega_{E,\rho,k}^+} \text{Re}(\eta_E(\omega, t)e^{j\sigma\omega t}) & \text{if } \delta(E) = N, \delta_k(E) \geq 1 \\ 0 & \text{if } \delta_k(E) = 0, \end{cases} \quad (9)$$

where  $\omega_E$  is a frequency and  $\Omega_{E,\rho,k}^+, \rho = 1, 2, \dots, |E|, k = 1, 2, \dots, M$ , is a set of frequencies we will specify later,  $\eta_{k,0} : \mathbb{R} \rightarrow \mathbb{R}, \eta_{E,k}(\omega, t), \eta_E(\omega, t) : \mathbb{R} \times \mathbb{R} \rightarrow \mathbb{C}$  are time-varying coefficients to be chosen and  $j$  is the imaginary unit. However, the superposition does not work as one would wish for but there are two issues one has to take care of:

1. The input sequences  $U_{k,E}^\sigma$  may not interfere with each other in a certain way to make sure that the superposition principle holds. This can be dealt with by a proper choice of the frequencies  $\omega_E$  and the sets of frequencies  $\Omega_{E,k}^+$ , see ["Choice of frequencies"](#).
2. Each input sequence  $U_{k,E}^\sigma$  not only excites the desired brackets  $E \cap \mathcal{B}$  but also all other equivalent brackets in  $E$ . We can overcome this by a proper choice of the coefficients  $\eta_{E,k}(\omega, t), \eta_E(\omega, t)$ , see ["Determining the coefficients"](#). The idea behind this is to intentionally also excite the undesired equivalent brackets, which itself excite the desired bracket, in such a way that the undesired equivalent brackets all cancel out.

Note that since the coefficients depends on the choice of frequencies, both issues cannot be handled separately but we first need to choose the frequencies to then be able to calculate corresponding coefficients. Observe further that if  $\delta(B) = 2$  then  $E(B) = B$  which makes the case of brackets of degree two particularly simple since we do not have to care about the second issue. In fact, it is  $|E(B)| \geq (\delta(B) - 1)!$  such that the higher the degree of the bracket to be excited, the more "undesired" equivalent brackets we need to take care of.

## 4. Reformulation of the algorithm

### 4.1. Reformulation of the inputs

We first show how to reformulate the approximating inputs proposed in [3] to obtain (7), (9). In [3], the approximating inputs take the form

$$U_k^\sigma(t) = \eta_{k,0}(t) + \sqrt{\sigma} \sum_{\omega \in \Omega(2,k)} \eta_{\omega,k}(t)e^{j\sigma\omega t} + \sum_{N=3}^r \sigma\frac{N-1}{N} \sum_{\omega \in \Omega(N,k)} \eta_\omega(t)e^{j\sigma\omega t}. \quad (10)$$

The following assumptions are imposed in [3] on the sets  $\Omega(N, k)$  and the time dependent coefficients  $\eta_{k,0}, \eta_{\omega,k}, \eta_\omega$ :

- [A1]** For  $N = 2, \dots, r, k = 1, \dots, M$ , the sets  $\Omega(N, k) \subset \mathbb{R} \setminus \{0\}$  are pairwise disjoint and finite.

[A2] Each  $\Omega(N, k)$  is symmetric, i.e.  $\omega \in \Omega(N, k)$  implies that  $-\omega \in \Omega(N, k)$ .

[A3] For  $k = 1, \dots, M$ , it is  $\eta_{\omega, k}, \eta_{\omega} : \mathbb{R} \rightarrow \mathbb{C}, \eta_{\omega, k}, \eta_{\omega} \in \mathcal{C}^1$ .

[A4] For  $k = 1, \dots, M$ , it is  $\eta_{0, k} : \mathbb{R} \rightarrow \mathbb{R}, \eta_{0, k} \in \mathcal{C}^1$ .

[A5] For each  $\omega \in \bigcup_{N=3}^r \bigcup_{k=1}^M \Omega(N, k)$  it is  $\eta_{-\omega}(t) = \overline{\eta_{\omega}(t)}$  for all  $t$ , and for  $\omega \in \Omega(2, k)$  for each  $k = 1, 2, \dots, M$  it is  $\eta_{-\omega, k}(t) = \overline{\eta_{\omega, k}(t)}$  for all  $t$ .

The sets  $\Omega(n, k)$  are then decomposed according to

$$\Omega(n, k) = \bigcup_{E \in \mathcal{E}_N} \bigcup_{\rho=1}^{|E|} \Omega_{E, \rho, k}, \quad (11)$$

where  $\mathcal{E}_N = \{E(B) : B \in \mathcal{B}, \delta(B) = N\}$  is the set of all equivalence classes of all brackets in  $\mathcal{B}$  of degree  $N$ . The following assumptions are then imposed on the sets  $\Omega_{E, \rho, k}$ :

[A6] For each  $E \in \bigcup_{N=2}^r \mathcal{E}_N, \rho = 1, 2, \dots, |E|, k = 1, 2, \dots, M$ , the set  $\Omega_{E, \rho, k} \subset \mathbb{R} \setminus \{0\}$  is symmetric and has cardinality  $|\Omega_{E, \rho, k}| = 2\delta_k(E)$ .

[A7] For each  $E \in \bigcup_{N=3}^r \mathcal{E}_N, \rho = 1, 2, \dots, |E|$ , the sets  $\Omega_{E, \rho, k}$  are pairwise disjoint when  $k = 1, 2, \dots, M$ .

[A8] For each  $E = [\phi_{k_1}, \phi_{k_2}] \in \mathcal{E}_2$  we have  $\Omega_{E, 1, k_1} = \Omega_{E, 1, k_2}$ .

[A9] For each  $E \in \bigcup_{N=3}^r \mathcal{E}_N, \rho = 1, 2, \dots, |E|$ , the set

$$\Omega_{E, \rho} = \bigcup_{k=1}^M \Omega_{E, \rho, k} \quad (12)$$

is symmetrically minimally canceling, see [Definition 2](#) for a definition.

[A10] The collection of sets

$$\{\Omega_{E, \rho}\}_{E \in \bigcup_{N=3}^r \mathcal{E}_N, \rho=1, 2, \dots, |E|} \quad (13)$$

is an independent collection, see [Definition 3](#) for a definition.

In the following we want to use some of these assumptions to reformulate the inputs (10). By [A2], it is  $\Omega(N, k) = \Omega^+(N, k) \cup \Omega^-(N, k)$  where we write  $\Omega^+(N, k)$  and  $\Omega^-(N, k)$  for the two disjoint symmetric components. Note that this does not mean that  $\omega > 0$  for

all  $\omega \in \Omega^+(N, k)$ . We then have

$$\begin{aligned}
U_k^\sigma(t) &= \eta_{k,0}(t) + \sqrt{\sigma} \sum_{\omega \in \Omega^+(2,k)} (\eta_{\omega,k}(t)e^{j\sigma\omega t} + \eta_{-\omega,k}(t)e^{-j\sigma\omega t}) \\
&\quad + \sum_{N=3}^r \sigma^{\frac{N-1}{N}} \sum_{\omega \in \Omega^+(N,k)} (\eta_{\omega}(t)e^{j\sigma\omega t} + \eta_{-\omega}(t)e^{-j\sigma\omega t}) \\
&= \eta_{k,0}(t) + 2\sqrt{\sigma} \sum_{\omega \in \Omega^+(2,k)} \operatorname{Re}(\eta_{\omega,k}(t)e^{j\sigma\omega t}) \\
&\quad + \sum_{N=3}^r 2\sigma^{\frac{N-1}{N}} \sum_{\omega \in \Omega^+(N,k)} \operatorname{Re}(\eta_{\omega}(t)e^{j\sigma\omega t})
\end{aligned} \tag{14}$$

where we used [A5] in the second step. Additionally, by [A10], we have that for each  $N = 3, \dots, r, k = 1, 2, \dots, M$ ,

$$\sum_{\omega \in \Omega^+(2,k)} \operatorname{Re}(\eta_{\omega,k}(t)e^{j\sigma\omega t}) = \sum_{E \in \mathcal{E}_2} \operatorname{Re}(\eta_{\omega_{E,1,k}}(t)e^{j\sigma\omega_{E,1,k}t}) \tag{15}$$

$$\sum_{\omega \in \Omega^+(N,k)} \operatorname{Re}(\eta_{\omega}(t)e^{j\sigma\omega t}) = \sum_{E \in \mathcal{E}_N} \sum_{\rho=1}^{|E|} \sum_{\omega \in \Omega_{E,\rho,k}^+} \operatorname{Re}(\eta_{\omega}(t)e^{j\sigma\omega t}), \tag{16}$$

where we used that for  $E \in \mathcal{E}_2$  it is  $|E| = 1$  such that [A6] implies that  $\Omega_{E,\rho,k} = \{\omega_{E,\rho,k}, -\omega_{E,\rho,k}\}$  with  $\rho = 1$  and we define  $\Omega_{E,\rho,k}^+ = \omega_{E,\rho,k}$ . Since  $E(B) = \{B\}$  for  $\delta(B) = 2$  and using [A8], for a simpler notation we let  $\omega_E := \omega_{E,1,k}$  for any  $E \in \mathcal{E}_2, k \in \{s : \delta_s(E) = 1\}$ . Note further that [A6] implies that  $\Omega_{E,\rho,k}^+ = \emptyset$  for any  $E$  with  $\delta_k(E) = 0$ . Using everything in the input (14) we hence obtain

$$\begin{aligned}
U_k^\sigma(t) &= \eta_{k,0}(t) + 2\sqrt{\sigma} \sum_{\substack{E \in \mathcal{E}_2: \\ \delta_k(E) \neq 0}} \operatorname{Re}(\eta_{\omega_E,k}(t)e^{j\sigma\omega_E t}) \\
&\quad + \sum_{N=3}^r 2\sigma^{\frac{N-1}{N}} \sum_{\substack{E \in \mathcal{E}_N: \\ \delta_k(E) \neq 0}} \sum_{\rho=1}^{|E|} \sum_{\omega \in \Omega_{E,\rho,k}^+} \operatorname{Re}(\eta_{\omega}(t)e^{j\sigma\omega t}).
\end{aligned} \tag{17}$$

Finally, making the change of notation

$$\eta_{\omega,k}(t) \rightsquigarrow \eta_{E,k}(\omega, t), \quad \eta_{\omega}(t) \rightsquigarrow \eta_E(\omega, t), \tag{18}$$

for any  $\omega \in \Omega_{E,\rho,k}$ , we see that (17) is exactly the same as (7) together with (9).

## 4.2. Choice of frequencies

Next, we reformulate the constraints [A1] - [A10]. Observe that by the reformulation of the inputs we have already incorporated [A2], [A3], [A4], [A5] and [A8] into (7), (9). In

view of [A6] we then let

$$\Omega_{E,\rho,k}^+ = \{\omega_{E,\rho,k,1}, \omega_{E,\rho,k,2}, \dots, \omega_{E,\rho,k,\delta_k(E)}\}. \quad (19)$$

We now sum up the remaining constraints on the set of frequencies:

**Assumption 1.** We impose the following assumptions on the sets of frequencies:

1. For each  $E \in \mathcal{E}$  with  $\delta(E) \geq 3$ ,  $\rho = 1, 2, \dots, |E|$ ,  $k = 1, 2, \dots, M$ , the frequencies  $\omega_{E,\rho,k,i}$ ,  $i = 1, 2, \dots, \delta_k(E)$ , are pairwise disjoint. ([A7])

2. For each  $E \in \mathcal{E}$ ,  $\delta(E) \geq 3$ , and each  $\rho = 1, \dots, |E|$ , the set

$$\Omega_{E,\rho}^+ = \bigcup_{k=1}^M \Omega_{E,\rho,k} \quad (20)$$

is *minimally canceling*. ([A9])

3. The collection of sets

$$\left\{ \{\omega_E, -\omega_E\}_{E \in \mathcal{E}_2}, \{\Omega_{E,\rho}^+ \cup \Omega_{E,\rho}^-\}_{E \in \mathcal{E}, \delta(E) \geq 3, \rho=1, \dots, |E(B)|} \right\} \quad (21)$$

is *independent*. ([A10])

Here, we made use of the following two definitions:

**Definition 2** (Minimally canceling). A set  $\Omega = \{\omega_1, \dots, \omega_m\}$  is called *minimally canceling* if for each collection of integers  $\{y_i\}_{i=1}^m$  such that  $\sum_{k=1}^m |y_k| \leq m$  it follows that  $\sum_{k=1}^m y_k \omega_k = 0$  if and only if all  $y_k$  are equal.

**Definition 3** (Independent collection). A finite collection of sets  $\{\Omega_\lambda\}_{\lambda=1}^N$ , where  $\Omega_\lambda = \{\omega_{\lambda,1}, \omega_{\lambda,2}, \dots, \omega_{\lambda,M_\lambda}\}$ , is called *independent* if the followings hold:

1. the sets  $\Omega_\lambda$  are pairwise disjoint, and
2. for each collection of integers  $\{y_{i,k}\}_{i=1}^N, k = 1, \dots, M_i$ , such that

$$\sum_{i=1}^N \sum_{k=1}^{M_i} y_{i,k} \omega_{i,k} = 0 \quad \text{and} \quad \sum_{i=1}^N \sum_{k=1}^{M_i} |y_{i,k}| \leq \sum_{i=1}^N M_i$$

we have

$$\sum_{k=1}^{M_i} y_{i,k} \omega_{i,k} = 0, \quad (22)$$

for each  $i = 1, 2, \dots, N$ .

While those conditions are not very restrictive as we will illustrate in the following, it is nevertheless hard to explicitly construct sets of frequencies that are ensured to fulfill them. We now first give an interpretation of [Definition 2](#). Alternatively representing the (ordered) set  $\{\omega_1, \dots, \omega_m\}$  as a vector  $\omega = [\omega_1, \omega_2, \dots, \omega_m]^\top \in \mathbb{R}^m$ , one can reformulate this definition in the following way: Let

$$\mathbb{Y} := \{y \in \mathbb{Z}^m : \sum_{k=1}^m |y_k| \leq m\}. \quad (23)$$

Then the maximal set of minimal canceling frequencies is given as

$$\begin{aligned} \Omega_{\max} &= \{\omega \in \mathbb{R}^m : \forall y \in \mathbb{Y} : \omega^\top y = 0 \Leftrightarrow y = c\mathbf{1}, c \in \mathbb{Z}\} \\ &= \{\omega \in \mathbb{R}^m : \omega^\top \mathbf{1}c = 0, \quad c \in \{-1, 0, 1\}, \\ &\quad \omega^\top y \neq 0 \quad \forall y \in \mathbb{Y} \setminus \{-\mathbf{1}, \mathbf{0}, \mathbf{1}\}\}, \end{aligned} \quad (24)$$

where  $\mathbf{0}, \mathbf{1} \in \mathbb{R}^m$  denote the vectors with all entries equal to zero and all entries equal to 1, respectively. Note that the first condition implies that for a set of frequencies to be minimally canceling it is necessary that

$$\omega_m = -\sum_{k=1}^{m-1} \omega_k. \quad (25)$$

Notice further that the set  $\Omega_{\max}$  is never empty since the first condition restricts the set to a hyperplane of dimension  $m - 1$  (the one that is orthogonal to the all ones vector) and the inequality constraints define a finite number of additional hyperplanes of dimension  $m - 1$  in which the  $\omega$  may not lie. Thus, the set  $\Omega$  is a hyperplane of dimension  $m - 1$  from which a finite set of  $m - 2$  dimensional hyperplanes is cut out. For  $m = 3$ , the situation is illustrated in [Figure 1](#). Hence, even though the number of inequality constraints might be large, the constraints are not restrictive.

### 4.3. The limiting system

In order to see how to choose the coefficients we first investigate the limiting behavior of the trajectories of (6) together with the inputs (7), (9) under the assumption that the frequencies fulfill [Assumption 1](#). According to [3, Theorem 8.1] and adopting to the previously defined notation, the trajectories of (6) together with inputs (7), (9) uniformly converge – for increasing  $\sigma$  and under [Assumption 1](#) – to the trajectories of

$$\begin{aligned} \dot{x} &= f_0(x) + \sum_{k=1}^M \eta_{k,0}(t) \phi_k(x) + \sum_{E(B)=\{B\} \in \mathcal{E}_2} \frac{1}{j\omega_E} \zeta_E(t) B(x) \\ &+ \sum_{n=3}^r \sum_{E \in \mathcal{E}_n} \sum_{B \in E} \sum_{\rho=1}^{|E|} j^{1-\delta(E)} \left( \sum_{F \in Q_{E,\rho}} \tilde{\zeta}_{B,\rho}^F \prod_{\omega \in F} \eta_E(\omega, t) \right) B(x), \end{aligned} \quad (26)$$



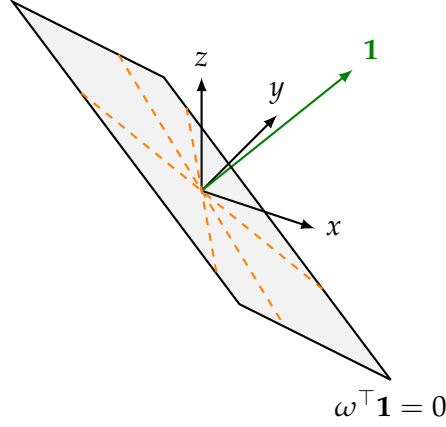

Figure 1: An illustration of the minimally canceling property for  $m = 3$ . The gray plane indicates the set of  $\omega$  for which  $\omega^\top \mathbf{1} = 0$ . The dashed orange lines indicate the intersection of this set with some of the planes defined by the second condition in (24). The set  $\Omega_{\max}$  is then the gray plane without the dashed orange lines. Apparently, since the number of those orange lines is possibly large but finite, if we randomly pick  $\omega$  in the gray plane the probability of obtaining a minimally canceling  $\omega$  is 1 almost surely.

where  $Q_{E,\rho} = \{\Omega_{E,\rho}^+, \Omega_{E,\rho}^-\}$  and where for  $E = \{B\} = \{[\phi_{k_1}, \phi_{k_2}]\}$  we have

$$\zeta_E(t) = \eta_{E,k_1}(\omega_E, t)\eta_{E,k_2}(-\omega_E, t) - \eta_{E,k_1}(-\omega_E, t)\eta_{E,k_2}(\omega_E, t) \quad (27)$$

and for  $B \in E$ ,  $\delta(E) \geq 3$ , it is

$$\tilde{\zeta}_{B,\rho}^F = g_B(F \cap \Omega_{E,\rho,1}, F \cap \Omega_{E,\rho,2}, \dots, F \cap \Omega_{E,\rho,M}) \quad (28)$$

with  $g_B$  being a recursively defined function that we will explain in the following. Keeping in mind the definition of  $Q_{E,\rho}$ , we first define

$$\tilde{\zeta}_{B,\rho}^+ := \tilde{\zeta}_{B,\rho}^{\Omega_{E,\rho}^+}, \quad \tilde{\zeta}_{B,\rho}^- := \tilde{\zeta}_{B,\rho}^{\Omega_{E,\rho}^-} \quad (29)$$

and observe that together with (12) as well as [A6] we have

$$F \cap \Omega_{E,\rho,k} = \begin{cases} \emptyset & \text{if } \delta_k(E) = 0 \\ \Omega_{E,\rho,k}^+ & \text{if } F = \Omega_{E,\rho}^+ \\ \Omega_{E,\rho,k}^- & \text{if } F = \Omega_{E,\rho}^- \end{cases} \quad (30)$$

where  $\Omega_{E,\rho,k}^+, \Omega_{E,\rho,k}^-$  are the symmetric components of  $\Omega_{E,\rho,k}$ . Hence, it is

$$\zeta_{B,\rho}^+ = g_B(\Omega_{E,\rho,1}^+, \Omega_{E,\rho,2}^+, \dots, \Omega_{E,\rho,M}^+), \quad (31)$$

$$\zeta_{B,\rho}^- = g_B(\Omega_{E,\rho,1}^-, \Omega_{E,\rho,2}^-, \dots, \Omega_{E,\rho,M}^-). \quad (32)$$

Let now  $\theta_B : \{1, 2, \dots, \delta(B)\} \rightarrow \{1, 2, \dots, M\}$  where  $\theta_B(i) = k$  if the vector field in the  $i$ -th place in the bracket  $B$  is  $\phi_k$ . For example, for  $B = [\phi_3, [\phi_1, \phi_2]]$  it is  $\theta_B(1) = 3$ ,  $\theta_B(2) = 1$  and  $\theta_B(3) = 2$ . Also, let  $\theta_B^{-1}(k) = \{s : \theta_B(s) = k\}$  denote the set of places in the bracket  $B$  with vector field  $\phi_k$ . Define  $\text{perm}(B)$  to be the set of all permutations of  $\{1, 2, \dots, \delta(B)\}$  that sort the set  $\{\theta_B(i)\}_{i=1,2,\dots,\delta(B)}$  in ascending order, or in more precise words, map the set  $\theta_B^{-1}(k)$  to the interval

$$\mathcal{I}_{B,k} = \left\{ \sum_{j=1}^{k-1} \delta_j(B) + 1, \dots, \sum_{j=1}^k \delta_j(B) \right\}. \quad (33)$$

We then define

$$g_B(\omega_1, \omega_2, \dots, \omega_{\delta(B)}) = \sum_{\pi \in \text{perm}(B)} \hat{g}_B(\omega_{\pi(1)}, \omega_{\pi(2)}, \dots, \omega_{\pi(\delta(B))}) \quad (34)$$

where  $\hat{g}_B$  is defined recursively as

- if  $\delta(B) = 1$ :

$$\hat{g}_B(\tilde{\omega}_1) = 1 \quad (35)$$

- if  $B = \text{ad}_{B_1}^\kappa(B_2) = [B_1, [B_1, \dots, [B_1, B_2] \dots]]$ :

$$\hat{g}_B(\tilde{\omega}_1, \tilde{\omega}_2, \dots, \tilde{\omega}_{\delta(B)}) = \frac{1}{\kappa} \hat{g}_{B_2}(\tilde{\omega}_{\kappa n_1+1}, \tilde{\omega}_{\kappa n_1+2}, \dots, \tilde{\omega}_{\kappa n_1+\delta(B_2)}) \quad (36)$$

$$\times \prod_{q=1}^{\kappa} \frac{\hat{g}_{B_2}(\tilde{\omega}_{(q-1)n_1+1}, \tilde{\omega}_{(q-1)n_1+2}, \dots, \tilde{\omega}_{qn_1})}{\sum_{i=1}^{n_1} \tilde{\omega}_{(q-1)n_1+i}} \quad (37)$$

where  $n_1 = \delta(B_1)$ ,  $n_2 = \delta(B_2)$ .

Observe now that these calculations simplify under the following assumption:

**Simplification 1.** Suppose that  $\delta_k(B) \in \{0, 1\}$  for all  $k = 1, 2, \dots, M$ , i.e., each vector field appears at most once in a bracket. Then the sets  $\Omega_{E,\rho,k}^+, \Omega_{E,\rho,k}^-$  are either empty or have cardinality one and  $\text{perm}(B)$  has only one element. Then it is

$$g_B(\omega_1, \omega_2, \dots, \omega_{\delta(B)}) = \hat{g}_B(\omega_{\theta_B(1)}, \omega_{\theta_B(2)}, \dots, \omega_{\theta_B(\delta(B))}) \quad (38)$$

and  $\kappa = 1$  in (37).

Note that this assumption holds in the motivating application [5].

We now use our definitions to rewrite the limiting system (26). Observe first that for  $F = \Omega_{E,\rho}^-$  we have

$$\prod_{\omega \in F} \eta_E(\omega, t) = \prod_{\omega \in \Omega_{E,\rho}^-} \eta_E(\omega, t) = \prod_{\omega \in \Omega_{E,\rho}^+} \eta_E(-\omega, t) = \prod_{\omega \in \Omega_{E,\rho}^+} \overline{\eta_E(\omega, t)} = \overline{\prod_{\omega \in \Omega_{E,\rho}^+} \eta_E(\omega, t)} \quad (39)$$

such that

$$\sum_{F \in Q_{E,\rho}} \zeta_{B,\rho}^F \prod_{\omega \in F} \eta_E(\omega, t) = \zeta_{B,\rho}^+ \prod_{\omega \in \Omega_{E,\rho}^+} \eta_E(\omega, t) + \zeta_{B,\rho}^- \overline{\prod_{\omega \in \Omega_{E,\rho}^+} \eta_E(\omega, t)}. \quad (40)$$

By the definition of  $\zeta_{B,\rho}^+$ ,  $\zeta_{B,\rho}^-$  it is

$$\zeta_{B,\rho}^+ = \begin{cases} \zeta_{B,\rho}^- & \text{if } \delta(B) \text{ is odd} \\ -\zeta_{B,\rho}^- & \text{if } \delta(B) \text{ is even} \end{cases} \quad (41)$$

such that

$$j^{1-\delta(E)} \sum_{F \in Q_{E,\rho}} \zeta_{B,\rho}^F \prod_{\omega \in F} \eta_E(\omega, t) = \zeta_{B,\rho}^+ \gamma_{E,\rho}(t) \quad (42)$$

where we defined

$$\gamma_{E,\rho}(t) := \begin{cases} 2^{j^{1-\delta(E)}} \operatorname{Re} \left( \prod_{\omega \in \Omega_{E,\rho}^+} \eta_E(\omega, t) \right) & \text{if } \delta(E) \text{ is odd} \\ 2^{j^{2-\delta(E)}} \operatorname{Im} \left( \prod_{\omega \in \Omega_{E,\rho}^+} \eta_E(\omega, t) \right) & \text{if } \delta(E) \text{ is even.} \end{cases} \quad (43)$$

Thus, we can rewrite (26) as

$$\begin{aligned} \dot{x} = & f_0(x) + \sum_{k=1}^M \eta_{k,0}(t) \phi_k(x) + \sum_{E(B)=\{B\} \in \mathcal{E}_2} \frac{1}{j\omega_E} \zeta_E(t) B(x) \\ & + \sum_{n=3}^r \sum_{E \in \mathcal{E}_n} \sum_{B \in E} \sum_{\rho=1}^{|E|} \zeta_{B,\rho}^+ \gamma_{E,\rho}(t) B(x). \end{aligned} \quad (44)$$

#### 4.4. Determining the coefficients

The idea to determine the coefficients  $\eta_{k,0}, \eta_{k,\omega}, \eta_\omega$  is then to choose them in such a way that the limiting system (44) matches the desired one given by (5). To this end, we first

rewrite (5) as

$$\dot{x} = f_0(x) + \sum_{n=1}^M v_{\phi_n}(t) \phi_n(x) + \sum_{E(B)=\{B\} \in \mathcal{E}_2} v_B(t) B(x) + \sum_{n=3}^{\delta_{\max}(B)} \sum_{E \in \mathcal{E}_n} \sum_{B \in E} v_B(t) B(x), \quad (45)$$

where  $v_B(t) \equiv 0$  for all  $B \in \mathcal{E} \setminus \mathcal{B}$ . Now, matching the dynamics (45) and (44), we obtain the following conditions:

- For  $\delta(B) = 1$  we require

$$v_B(t) = v_{\phi_k}(t) = \eta_{k,0}(t). \quad (46)$$

- For  $\delta(B) = 2$ , we require

$$v_B(t) = \zeta_{E(B)}(t) \quad (47)$$

- For  $\delta(B) \geq 3$  we require for each  $B \in E$

$$v_B(t) = \sum_{\rho=1}^{|E|} \zeta_{B,\rho}^+ \gamma_{E,\rho}(t), \quad (48)$$

i.e., if  $E = \{\tilde{B}_1, \tilde{B}_2, \dots, \tilde{B}_{|E|}\}$  with  $B_1 = B$ , this amounts to solving the quadratic system of linear equations

$$\underbrace{\begin{bmatrix} \zeta_{\tilde{B}_1,1}^+ & \zeta_{\tilde{B}_1,2}^+ & \cdots & \zeta_{\tilde{B}_1,|E|}^+ \\ \zeta_{\tilde{B}_2,1}^+ & \zeta_{\tilde{B}_2,2}^+ & \cdots & \zeta_{\tilde{B}_2,|E|}^+ \\ \vdots & \vdots & \ddots & \vdots \\ \zeta_{\tilde{B}_{|E|},1}^+ & \zeta_{\tilde{B}_{|E|},2}^+ & \cdots & \zeta_{\tilde{B}_{|E|},|E|}^+ \end{bmatrix}}_{=: \Xi_E} \begin{bmatrix} \gamma_{E,1}(t) \\ \gamma_{E,2}(t) \\ \vdots \\ \gamma_{E,|E|}(t) \end{bmatrix} = \begin{bmatrix} v_{\tilde{B}_1}(t) \\ v_{\tilde{B}_2}(t) \\ \vdots \\ v_{\tilde{B}_{|E|}}(t) \end{bmatrix}. \quad (49)$$

It has been shown in [3] that there always exists a choice of frequencies that fulfills the previously discussed assumption such that the matrix  $\Xi_E$  is non-singular; hence the required  $\gamma_{E,i}(t)$  can be computed from this equation.

While (46) obviously lets no degree of freedom, by (27) and (43) there are multiple possible choices in terms of the coefficients  $\eta_{E,k}(\omega, t)$ ,  $\eta_E(\omega, t)$  to fulfill (47) and (49). A particularly simple choice is presented in [3] and we generalize this in the following.

Before we present suitable choices of the coefficients we discuss a simplification that is of drastic importance in the application [5]. Obviously, with (49) we need to solve a system of linear equations of size equal to the cardinality of the equivalence class which grows rapidly with the degree of the bracket such that this might become computationally heavy quite fast. Additionally, one needs to compute  $|E|^2$  entries of the matrix  $\Xi_E$  by the recursion. However, if some of the brackets in the equivalence class evaluate to zero or are linearly dependent for a given set of vector fields  $\Phi$ , the

computational effort might be reduced since one only needs to consider a subset of each equivalence class  $E$  in (44), thus also the number of conditions reduces.

**Simplification 2.** *Let*

$$E_0(B) := \{\tilde{B} \in E(B) : \tilde{B}(x) = 0 \text{ for all } x \in \mathbb{R}^n\} \quad (50)$$

$$E_{\text{red}}(B) := E(B) \setminus E_0(B) \quad (51)$$

and suppose w.l.o.g. that  $E_{\text{red}}(B) = \{\tilde{B}_1, \tilde{B}_2, \dots, \tilde{B}_{|E_{\text{red}}(B)|}\}$ . Then the condition (49) for  $\gamma_{E,i}$ ,  $i = 1, 2, \dots, |E_{\text{red}}(B)|$ , reduces to

$$\underbrace{\begin{bmatrix} \zeta_{\tilde{B}_1,1}^+ & \zeta_{\tilde{B}_1,2}^+ & \cdots & \zeta_{\tilde{B}_1,|E_{\text{red}}(B)|}^+ \\ \zeta_{\tilde{B}_2,1}^+ & \zeta_{\tilde{B}_2,2}^+ & \cdots & \zeta_{\tilde{B}_2,|E_{\text{red}}(B)|}^+ \\ \vdots & \vdots & \ddots & \vdots \\ \zeta_{\tilde{B}_{|E_{\text{red}}(B)|},1}^+ & \zeta_{\tilde{B}_{|E_{\text{red}}(B)|},2}^+ & \cdots & \zeta_{\tilde{B}_{|E_{\text{red}}(B)|},|E_{\text{red}}(B)|}^+ \end{bmatrix}}_{=:\Xi_{E_{\text{red}}(B)}} \begin{bmatrix} \gamma_{E,1}(t) \\ \gamma_{E,2}(t) \\ \vdots \\ \gamma_{E,|E_{\text{red}}(B)|}(t) \end{bmatrix} = \begin{bmatrix} v_{\tilde{B}_1}(t) \\ v_{\tilde{B}_2}(t) \\ \vdots \\ v_{\tilde{B}_{|E_{\text{red}}(B)|}}(t) \end{bmatrix} \quad (52)$$

and  $\gamma_{E,i}$ ,  $i = |E_{\text{red}}(B)| + 1, \dots, |E(B)|$ , is arbitrary.

In general situations the reduction in computational effort might be small, but in several application scenarios  $|E_0(B)| \gg |E_{\text{red}}(B)|$  such that (52) is much simpler to obtain and solve than (49). For example, this is the case in the application considered in [5], cf. Figure 2.

It should as well be noted that **Simplification 2** does not need any assumptions and thus can be always used, while not being helpful in any case. We next elaborate on how to choose the coefficients  $\eta_{E,k}(\omega, t)$ ,  $\eta_E(\omega, t)$  from (47) and (52).

**Choice of  $\eta_{E,k}(\omega, t)$**  For all equivalence classes  $E = \{B = [\phi_{k_1}, \phi_{k_2}]\} \in \mathcal{E}_2$ , we propose to choose

$$\eta_{E,k_1}(\omega_E, t) = j \frac{1}{\beta_B(t)} \sqrt{\frac{1}{2} v_B(t) \omega_E} \quad (53)$$

$$\eta_{E,k_2}(\omega_E, t) = \beta_B(t) \sqrt{\frac{1}{2} v_B(t) \omega_E}, \quad (54)$$

where  $\beta_B : \mathbb{R} \rightarrow \mathbb{C}$ ,  $\beta_B(t) \neq 0$  for all  $t$ , can be chosen freely. Observe that the choice proposed in [3, CH3] is a special case and corresponds to taking  $\beta_B(t) = \sqrt{\frac{1}{2} v_B(t) \omega_E}$ . Our choice allows to "distribute" the perturbations between the inputs  $u_{k_1}, u_{k_2}$ , or in other words, to the vector fields  $\phi_{k_1}, \phi_{k_2}$ .

**Choice of  $\eta_E(\omega, t)$**  We suggest the following choice:

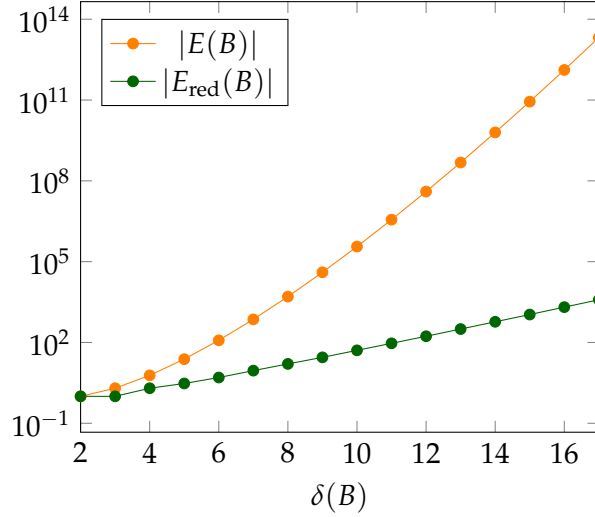

| $\delta(B)$    | 2 | 3 | 4  | 5  | 6  | 7  | 8  | 9  | 10 | 11  | 12  | 13  | 14  | 15   | 16   | 17!  |
|----------------|---|---|----|----|----|----|----|----|----|-----|-----|-----|-----|------|------|------|
| $ E(B) $       | 1 | 2 | 3! | 4! | 5! | 6! | 7! | 8! | 9! | 10! | 11! | 12! | 13! | 14!  | 15!  | 16!  |
| $ E_{\pm}(B) $ | 1 | 1 | 2  | 3  | 5  | 9  | 16 | 28 | 51 | 93  | 170 | 315 | 585 | 1089 | 2048 | 3855 |

Figure 2: A comparison of  $|E_0(B)|$  and  $|E_{\text{red}}(B)|$  for the application considered in [5]. The numbers were obtained by symbolically computing the resulting vector fields using a computer algebra system.

- If  $\delta(E)$  is odd, take

$$\eta_E(\omega, t) = \beta_{E,\omega} \left( \frac{1}{2} \gamma_{E,\rho}(t) j^{\delta(E)-1} \right)^{\frac{1}{\delta(E)}} \quad (55)$$

for all  $\omega \in \Omega_{E,\rho}^+$ , where  $\beta_{E,\omega} \in \mathbb{R}$  fulfills  $\prod_{\omega \in \Omega_{E,\rho}^+} \beta_{E,\omega} = 1$ .

- If  $\delta(E)$  is even, take

$$\eta_E(\omega, t) = j \beta_{E,\omega} \text{sign}(\gamma_{E,\rho}(t) j^{\delta(B)-2}) \left| \frac{1}{2} \gamma_{E,\rho}(t) j^{\delta(B)-2} \right|^{\frac{1}{\delta(B)}} \quad \text{for } \omega = \tilde{\omega} \quad (56)$$

$$\eta_E(\omega, t) = \beta_{E,\omega} \left| \frac{1}{2} \gamma_{E,\rho}(t) j^{\delta(B)-2} \right|^{\frac{1}{\delta(B)}} \quad \text{for } \omega \in \Omega_{E,\rho}^+ \setminus \{\tilde{\omega}\} \quad (57)$$

for some  $\tilde{\omega} \in \Omega_{E,\rho}^+$ , and where again  $\beta_{E,\omega} \in \mathbb{R}$  fulfills  $\prod_{\omega \in \Omega_{E,\rho}^+} \beta_{E,\omega} = 1$ .

The idea of choosing the scaling  $\beta_{E,\omega}$ , which can in principle also be chosen as time-varying functions, is again to distribute the perturbations amongst the different inputs or vector fields. The relation of  $\beta_{E,\omega}$  comes from the fact that  $\Omega_{E,\rho}^+ = \bigcup_{k=1}^M \Omega_{E,\rho,k}^+$  i.e., the

scaling  $\beta_{E,\omega}$  with  $\omega \in \Omega_{E,\rho,k}^+$  belongs to the  $k$ th input.

## 5. The algorithm

In the following we sum up the previous discussions in an algorithmic fashion. For interested readers we also provide a MATLAB implementation which has been specifically designed for the application in [5].

### 5.1. No additional assumptions

#### Algorithm

**Input** A P. Hall basis  $\mathcal{PH} = (\mathcal{P}, \prec)$  of a set of vector fields  $\Phi = \{\phi_1, \dots, \phi_M\}$ ,  
a set of brackets  $\mathcal{B} \in \mathcal{P}$   
and corresponding coefficients  $v_B : \mathbb{R} \rightarrow \mathbb{R}$ .

**Output** A set of input sequences  $U_k^\sigma, k = 1, 2, \dots, M$ .

1. For all  $B \in \mathcal{B}$ , determine the associated (reduced) equivalence class

$$E(B) = \{\tilde{B} \in \mathcal{P} : \tilde{B} \sim B, \tilde{B}(z) \neq 0\} = \{\tilde{B}_{E,1}, \tilde{B}_{E,2}, \dots, \tilde{B}_{E,|E(B)|}\}, \quad \tilde{B}_{E,1} = B$$

and let  $\mathcal{E} = \{E(B), B \in \mathcal{B}\}$ ,  $\mathcal{E}_i = \{E(B), B \in \mathcal{B} : \delta(E) = i\}$ .

2. For all  $E \in \mathcal{E}$ ,  $\delta(E) = 2$   
choose  $|\mathcal{E}_2|$  distinct frequencies  $\omega_E \in \mathbb{R}$ ,

and, for all  $E \in \mathcal{E}$ ,  $\delta(E) \geq 3$   
choose  $|E|$  sets

$$\begin{aligned} \Omega_{E,\rho,k} &= \{\Omega_{E,\rho,k'}^+, \Omega_{E,\rho,k'}^-\} \\ \Omega_{E,\rho,k}^+ &= \begin{cases} \{\omega_{E,\rho,k,1}, \dots, \omega_{E,\rho,k,i}\} & \text{if } \delta_k(E) = i \geq 1 \\ \emptyset & \text{if } \delta_k(E) = 0 \end{cases} \quad \begin{matrix} k = 1, \dots, M \\ \rho = 1, \dots, |E(B)| \end{matrix} \\ \Omega_{E,\rho,k}^- &= -\Omega_{E,\rho,k}^+ \end{aligned}$$

such that [Assumption 1](#) is fulfilled, i.e.

- a) For each  $E \in \mathcal{E}$  with  $\delta(E) \geq 3$ ,  $\rho = 1, 2, \dots, |E|$ ,  $k = 1, 2, \dots, M$ , the frequencies  $\omega_{E,\rho,k,i}$ ,  $i = 1, 2, \dots, \delta_k(E)$ , are pairwise disjoint.
- b) For each  $E \in \mathcal{E}$ ,  $\delta(E) \geq 3$ , and each  $\rho = 1, \dots, |E|$ , the set

$$\Omega_{E,\rho}^+ = \bigcup_{k=1}^M \Omega_{E,\rho,k}^+ \quad (58)$$

is **minimally canceling**.

c) The collection of sets

$$\left\{ \left\{ \omega_E, -\omega_E \right\}_{E \in \mathcal{E}_2}, \left\{ \Omega_{E,\rho}^+ \cup \Omega_{E,\rho}^- \right\}_{E \in \mathcal{E}, \delta(E) \geq 3, \rho=1, \dots, |E(B)|} \right\} \quad (59)$$

is **independent**.

3. For all  $E \in \mathcal{E}$  with  $\delta(E) \geq 3$ , compute

$$\Xi_E = \begin{bmatrix} \zeta_{\tilde{B}_{E,1},1}^+ & \zeta_{\tilde{B}_{E,1},2}^+ & \cdots & \zeta_{\tilde{B}_{E,1},|E|}^+ \\ \zeta_{\tilde{B}_{E,2},1}^+ & \zeta_{\tilde{B}_{E,2},2}^+ & \cdots & \zeta_{\tilde{B}_{E,2},|E|}^+ \\ \vdots & \vdots & \ddots & \vdots \\ \zeta_{\tilde{B}_{E,|E|},1}^+ & \zeta_{\tilde{B}_{E,|E|},2}^+ & \cdots & \zeta_{\tilde{B}_{E,|E|},|E|}^+ \end{bmatrix}, \quad (60)$$

where

$$\zeta_{B,\rho}^+ = g_B(\Omega_{E,\rho,1}^+, \Omega_{E,\rho,2}^+, \dots, \Omega_{E,\rho,M}^+) \quad (61)$$

with  $g_B$  defined according to (34).

4. For all  $E \in \mathcal{E}$  with  $\delta(E) = 2$ , i.e.,  $E(B) = \{B\} = [\phi_{k_1}, \phi_{k_2}]$ , set

$$\eta_{E,k_1}(\omega_E, t) = j \frac{1}{\beta_B(t)} \sqrt{\frac{1}{2} v_B(t) \omega_E} \quad (62)$$

$$\eta_{E,k_2}(\omega_E, t) = \beta_B(t) \sqrt{\frac{1}{2} v_B(t) \omega_E}, \quad (63)$$

where  $\beta_B : \mathbb{R} \rightarrow \mathbb{C}$ ,  $\beta_B(t) \neq 0$  for all  $t$ .

For all  $E \in \mathcal{E}$  with  $\delta(E) \geq 3$  let

$$\begin{bmatrix} \gamma_{E,1}(t) \\ \gamma_{E,2}(t) \\ \vdots \\ \gamma_{E,|E|}(t) \end{bmatrix} = \Xi_E^{-1} \begin{bmatrix} v_{\tilde{B}_{E,1}}(t) \\ v_{\tilde{B}_{E,2}}(t) \\ \vdots \\ v_{\tilde{B}_{E,|E|}}(t) \end{bmatrix} \quad (64)$$

and, for each  $\rho = 1, 2, \dots, |E|$ ,  $\omega \in \Omega_{E,\rho}^+$ , set

- If  $\delta(E)$  is odd, take

$$\eta_E(\omega, t) = \beta_{E,\omega} \left( \frac{1}{2} \gamma_{E,\rho}(t) j^{\delta(E)-1} \right)^{\frac{1}{\delta(E)}} \quad (65)$$

for all  $\omega \in \Omega_{E,\rho}^+$ , where  $\beta_{E,\omega} \in \mathbb{R}$  fulfills  $\prod_{\omega \in \Omega_{E,\rho}^+} \beta_{E,\omega} = 1$ .



- If  $\delta(E)$  is even, take

$$\eta_E(\omega, t) = j\beta_{E,\omega} \text{sign}(\gamma_{E,\rho}(t)j^{\delta(B)}) \left| \frac{1}{2}\gamma_{E,\rho}(t)j^{\delta(B)} \right|^{\frac{1}{\delta(B)}} \quad \text{for } \omega = \tilde{\omega} \quad (66)$$

$$\eta_E(\omega, t) = \beta_{E,\omega} \left| \frac{1}{2}\gamma_{E,\rho}(t)j^{\delta(B)} \right|^{\frac{1}{\delta(B)}} \quad \text{for } \omega \in \Omega_{E,\rho}^+ \setminus \{\tilde{\omega}\} \quad (67)$$

for some  $\tilde{\omega} \in \Omega_{E,\rho}^+$ . and where again  $\beta_{E,\omega} \in \mathbb{R}$  fulfills  $\prod_{\omega \in \Omega_{E,\rho}^+} \beta_{E,\omega} = 1$ .

5. Set

$$U_{k,E}^\sigma(t) = \begin{cases} v_B(t) & \text{if } \delta(E) = 1, \delta_k(E) = 1, E = B \\ 2\sqrt{\sigma} \text{Re}(\eta_{E,k}(\omega_E, t)e^{j\sigma\omega_E t}) & \text{if } \delta(E) = 2, \delta_k(E) = 1 \\ 2\sigma^{\frac{N-1}{N}} \sum_{\rho=1}^{|E|} \sum_{\omega \in \Omega_{E,\rho,k}^+} \text{Re}(\eta_E(\omega, t)e^{j\sigma\omega t}) & \text{if } \delta(E) = N, \delta_k(E) \geq 1 \\ 0 & \text{if } \delta_k(E) = 0, \end{cases} \quad (68)$$

## 5.2. With Simplification 1

### Algorithm

**Input** A P. Hall basis  $\mathcal{PH} = (\mathcal{P}, \prec)$  of a set of vector fields  $\Phi = \{\phi_1, \dots, \phi_M\}$ , a set of brackets  $\mathcal{B} \in \mathcal{P}$  with  $\delta_k(B) \in \{0, 1\}$  for all  $k, B \in \mathcal{B}$  and corresponding coefficients  $v_B : \mathbb{R} \rightarrow \mathbb{R}$ .

**Output** A set of input sequences  $U_k^\sigma, k = 1, 2, \dots, M$ .

1. For all  $B \in \mathcal{B}$ , determine the associated (reduced) equivalence class

$$E(B) = \{\tilde{B} \in \mathcal{P} : \tilde{B} \sim B, \tilde{B}(z) \neq 0\} = \{\tilde{B}_{E,1}, \tilde{B}_{E,2}, \dots, \tilde{B}_{E,|E(B)|}\}, \quad \tilde{B}_{E,1} = B$$

and let  $\mathcal{E} = \{E(B), B \in \mathcal{B}\}$ ,  $\mathcal{E}_i = \{E(B), B \in \mathcal{B} : \delta(E) = i\}$ .

2. For all  $E \in \mathcal{E}$ ,  $\delta(E) = 2$

choose  $|\mathcal{E}_2|$  distinct frequencies  $\omega_E \in \mathbb{R}$ ,

and, for all  $E \in \mathcal{E}$ ,  $\delta(E) \geq 3$

choose  $|E|$  sets

$$\begin{aligned}\Omega_{E,\rho,k} &= \{\Omega_{E,\rho,k}^+, \Omega_{E,\rho,k}^-\} \\ \Omega_{E,\rho,k}^+ &= \begin{cases} \omega_{E,\rho,k} & \text{if } \delta_k(E) = 1 \\ \emptyset & \text{if } \delta_k(E) = 0 \end{cases} \quad \begin{matrix} k = 1, \dots, M \\ \rho = 1, \dots, |E(B)| \end{matrix} \\ \Omega_{E,\rho,k}^- &= -\Omega_{E,\rho,k}^+\end{aligned}$$

such that **Assumption 1** is fulfilled, i.e.

a) For each  $E \in \mathcal{E}$ ,  $\delta(E) \geq 3$ , and each  $\rho = 1, \dots, |E|$ , the set

$$\Omega_{E,\rho}^+ = \bigcup_{k=1}^M \Omega_{E,\rho,k}^+$$

is **minimally canceling**.

b) The collection of sets

$$\left\{ \{\omega_E, -\omega_E\}_{E \in \mathcal{E}_2}, \{\Omega_{E,\rho}^+ \cup \Omega_{E,\rho}^-\}_{E \in \mathcal{E}, \delta(E) \geq 3, \rho=1, \dots, |E(B)|} \right\}$$

is **independent**.

3. For all  $E \in \mathcal{E}$  with  $\delta(E) \geq 3$ , compute

$$\Xi_E = \begin{bmatrix} \zeta_{\tilde{B}_{E,1},1}^+ & \zeta_{\tilde{B}_{E,1},2}^+ & \cdots & \zeta_{\tilde{B}_{E,1},|E|}^+ \\ \zeta_{\tilde{B}_{E,2},1}^+ & \zeta_{\tilde{B}_{E,2},2}^+ & \cdots & \zeta_{\tilde{B}_{E,2},|E|}^+ \\ \vdots & \vdots & \ddots & \vdots \\ \zeta_{\tilde{B}_{E,|E|},1}^+ & \zeta_{\tilde{B}_{E,|E|},2}^+ & \cdots & \zeta_{\tilde{B}_{E,|E|},|E|}^+ \end{bmatrix},$$

where

$$\zeta_{B,\rho}^+ = \hat{g}_B(\omega_{E,\rho,\theta_B(1)}, \omega_{E,\rho,\theta_B(2)}, \dots, \omega_{E,\rho,\theta_B(\delta(B))})$$

with  $\theta_B(i) = k$  if the  $i$ th vector field in  $B$  is  $\phi_k$  and where

- if  $\delta(B) = 1$ :

$$\hat{g}_B(\tilde{\omega}_1) = 1$$

- if  $B = [B_1, B_2]$ ,  $n_1 = \delta(B_1)$ ,  $n_2 = \delta(B_2)$ :

$$\hat{g}_B(\tilde{\omega}_1, \tilde{\omega}_2, \dots, \tilde{\omega}_{\delta(B)}) = \hat{g}_{B_2}(\tilde{\omega}_{n_1+1}, \tilde{\omega}_{n_1+2}, \dots, \tilde{\omega}_{n_1+\delta(B_2)}) \frac{\hat{g}_{B_1}(\tilde{\omega}_1, \tilde{\omega}_2, \dots, \tilde{\omega}_{n_1})}{\sum_{i=1}^{n_1} \tilde{\omega}_i}$$

4. For all  $E \in \mathcal{E}$  with  $\delta(E) = 2$ , i.e.,  $E(B) = \{B\} = [\phi_{k_1}, \phi_{k_2}]$ , set

$$\begin{aligned}\eta_{E,k_1}(\omega_E, t) &= j \frac{1}{\beta_B(t)} \sqrt{\frac{1}{2} v_B(t) \omega_E} \\ \eta_{E,k_2}(\omega_E, t) &= \beta_B(t) \sqrt{\frac{1}{2} v_B(t) \omega_E},\end{aligned}$$

where  $\beta_B : \mathbb{R} \rightarrow \mathbb{C}$ ,  $\beta_B(t) \neq 0$  for all  $t$ .

For all  $E \in \mathcal{E}$  with  $\delta(E) \geq 3$  let

$$\begin{bmatrix} \gamma_{E,1}(t) \\ \gamma_{E,2}(t) \\ \vdots \\ \gamma_{E,|E|}(t) \end{bmatrix} = \Xi_E^{-1} \begin{bmatrix} v_{B_{E,1}}(t) \\ 0 \\ \vdots \\ 0 \end{bmatrix}$$

and, for each  $\rho = 1, 2, \dots, |E|$ ,  $\omega \in \Omega_{E,\rho}^+$ , set

- If  $\delta(E)$  is odd, take

$$\eta_E(\omega, t) = \beta_{E,\omega} \left( \frac{1}{2} \gamma_{E,\rho}(t) j^{\delta(E)-1} \right)^{\frac{1}{\delta(E)}}$$

for all  $\omega \in \Omega_{E,\rho}^+$ , where  $\beta_{E,\omega} \in \mathbb{R}$  fulfills  $\prod_{\omega \in \Omega_{E,\rho}^+} \beta_{E,\omega} = 1$ .

- If  $\delta(E)$  is even, take

$$\begin{aligned}\eta_E(\omega, t) &= j \beta_{E,\omega} \text{sign}(\gamma_{E,\rho}(t) j^{\delta(B)}) \left| \frac{1}{2} \gamma_{E,\rho}(t) j^{\delta(B)} \right|^{\frac{1}{\delta(B)}} \quad \text{for } \omega = \tilde{\omega} \\ \eta_E(\omega, t) &= \beta_{E,\omega} \left| \frac{1}{2} \gamma_{E,\rho}(t) j^{\delta(B)} \right|^{\frac{1}{\delta(B)}} \quad \text{for } \omega \in \Omega_{E,\rho}^+ \setminus \{\tilde{\omega}\}\end{aligned}$$

for some  $\tilde{\omega} \in \Omega_{E,\rho}^+$ . and where again  $\beta_{E,\omega} \in \mathbb{R}$  fulfills  $\prod_{\omega \in \Omega_{E,\rho}^+} \beta_{E,\omega} = 1$ .

5. Set

$$U_{k,E}^\sigma(t) = \begin{cases} v_B(t) & \text{if } \delta(E) = 1, \delta_k(E) = 1, E = B \\ 2\sqrt{\sigma} \text{Re}(\eta_{E,k}(\omega_E, t) e^{j\sigma\omega_E t}) & \text{if } \delta(E) = 2, \delta_k(E) = 1 \\ 2\sigma^{\frac{N-1}{N}} \sum_{\rho=1}^{|E|} \sum_{\omega \in \Omega_{E,\rho,k}^+} \text{Re}(\eta_E(\omega, t) e^{j\sigma\omega t}) & \text{if } \delta(E) = N, \delta_k(E) \geq 1 \\ 0 & \text{if } \delta_k(E) = 0, \end{cases}$$

## A. Appendix

**Definition 4** (P. Hall basis of a Lie algebra). Let  $\Phi = \{\phi_1, \phi_2, \dots, \phi_m\}$  be a set of vector fields. A P. Hall basis  $\mathcal{PH}(\Phi) = (\mathbb{P}, \prec)$  of the Lie algebra of  $\Phi$  is a set  $\mathbb{P}$  of brackets equipped with a total ordering  $\prec$  that fulfills the following properties:

[PH1] Every  $\phi_k$  is in  $\mathbb{P}$ .

[PH2]  $\phi_k \prec \phi_j$  if and only if  $k < j$ .

[PH3] If  $B_1, B_2 \in \mathbb{P}$  and  $\delta(B_1) < \delta(B_2)$ , then  $B_1 \prec B_2$ .

[PH4] Each  $B = [B_1, B_2] \in \mathbb{P}$  if and only if

[PH4.a]  $B_1, B_2 \in \mathbb{P}$  and  $B_1 \prec B_2$

[PH4.b] either  $\delta(B_2) = 1$  or  $B_2 = [B_3, B_4]$  for some  $B_3, B_4$  such that  $B_3 \preceq B_1$ .

## References

- [1] Hans-Bernd Dürr, Milos S. Stankovic, Christian Ebenbauer, and Karl Henrik Johansson. Lie bracket approximation of extremum seeking systems. *Automatica*, 49(6):1538–1552, 2013.
- [2] C. Ebenbauer, S. Michalowsky, V. Grushkovskaya, and B. Gharesifard. Distributed optimization over directed graphs with the help of Lie brackets. In *Proc. 20th IFAC World Congress*, pages 15908–15913, 2017.
- [3] Wensheng Liu. An approximation algorithm for nonholonomic systems. *SIAM Journal on Control and Optimization*, 35(4):1328–1365, 1997.
- [4] S. Michalowsky, B. Gharesifard, and C. Ebenbauer. Distributed extremum seeking over directed graphs. In *Proc. 56th IEEE Conf. Decision and Control (CDC)*, pages 2095–2101, 2017.
- [5] S. Michalowsky, B. Gharesifard, and C. Ebenbauer. A Lie bracket approximation approach to distributed optimization over directed graphs. *ArXiv e-prints arXiv:1711.05486*, 2017. <https://arxiv.org/abs/1711.05486>.
- [6] Héctor J Sussmann and Wensheng Liu. Limits of highly oscillatory controls and the approximation of general paths by admissible trajectories. In *Decision and Control, 1991., Proceedings of the 30th IEEE Conference on*, pages 437–442. IEEE, 1991.
